# Supplementary material for: Resource-Aware Heterogeneous Federated Learning using Neural Architecture Search
Source: arXiv:2211.05716 source file (2024-05-01)
Supplement: Supplementary file 1 [file 07_supplementary_materials.tex]

\newpage
\onecolumn
\section{\centering{Supplementary experimental results}}

\label{sec:appendix}

\subsection{Summary}
In supplementary materials, we explore the cases where \proj fails to outperform baselines. This is quite expected as every design has its own strengths and weakness. There is no singular solution that universally addresses all possible FL settings.
We summarized scenarios where \proj shows in advanced: 
1. bandwidth matters.
2. public data available  
3. edge devices are resource limited.
4. large scale.

\subsection{Experiments}
We conducted extensive experiments to evaluate \proj and summarized our experiments into five sections: learning efficiency, communication efficiency, system heterogeneity, resource utilization, and ablation study.
In learning efficiency, we analyze the optimization ability for training the target model. The communication efficiency experiment investigates the communication cost incurred by client-server updates. 
In our system heterogeneity experiment, we highlight the advantage of \proj across systems with varying resources. %in different system hetero settings.
In the utilization experiment, we measure the overall resource use efficiency. Lastly, we conduct a comprehensive ablation study.

\subsection{Experimental Setup}
% \noindent\textbf{Datasets and models.} We conduct experiments on datasets inline with baselines: CIFAR-10/100~\cite{krizhevsky2009cifar}, FEMNIST~\cite{caldas2019leaf} and Tiny ImageNet~\cite{russakovsky2015imagenet} under Non-IID benchmark settings~\cite{li2022niidbench}. 
% We deploy resource-aware deep learning models sampled from MobileNetV2/V3~\cite{howard18mobilenetv2,howard19mobilenetv3} or ResNet \cite{he2016resnet} super-network in different cases. 
% Two popular datasets in the field: Cifar-10/100~\cite{krizhevsky2009cifar} and FEMNIST~\cite{caldas2019leaf} are used for training on local client. 
% In the non-IID setting, each client is assigned a sample proportion of each label based on the Dirichlet distribution (with concentration $\alpha$). Specifically, we sample $p_k \sim Dir_N(\alpha)$ and assign a $p_{k,j}$ proportion of the instances to client $j$. Here we choose the $\alpha = 0.1$. 
% In contrast, in baselines, we deploy a uniformed architecture sampled from MobileNetV2/V3 and ResNet correspondingly.
To avoid confusion, we identify networks by their capacity~(via FLOPs), eg. we identify ResNet-34 as: ResNet with $76$ MFLOPs.
% Additionally, our experiments also involve traditionally over-parameterized models, such as VGG-11/16~\cite{simonyan2015vgg}, for highlight comparison.
\\
\textbf{FL and Non-IID settings.} All our experiments are conducted on benchmark Non-IID settings~\cite{li2022niidbench}. 
Specifically, we use label heterogeneity to set up Non-IID.
We consider the following three scenarios: (a) traditional FL setting, (b) public data with ensemble knowledge distillation, and (c) transfer learning with NAS. 
With CIFAR-10/100, we experiment on different number of clients from $30$ to $100$ and sample $10\%$ to $70\%$ clients for communication, while with FEMNIST, we experiment on $3000$ clients.  \\
\textbf{Public data settings.} We tried different public data to perform ensemble distillation, including 10k randomly unlabled data points sampled from Tiny ImageNet, 10k randomly unlabled data points sampled from CINIC-10 (after removing overlaping with cifar-10), and 5k data points split from CIFAR-10 training data.
\\
\textbf{NAS settings.} We conduct neural architecture search on pre-trained OFA~\cite{cai20ofa} super-networks on ImageNet~\cite{russakovsky2015imagenet}. Super-network architectures involved in the experiments include ResNet, MobileNetV2, and MobileNetV3. Resource-aware models will be sampled from the super-networks. According to the FL settings, pre-trained weights inherited from super-network can be reset or transferred accordingly.
% the resource constraints, different sub-network will be selected from those super-network to each local devices. 
Detailed information is specified in the subsections. \\
\textbf{Knowledge Network setting.} We sampled a tiny network (in terms of FLOPs) from super-network as the knowledge network. 
In \proj, the network capacity we shows are the integrated capacity of knowledge network and specialized local network. For instance, we deploy a 30 MFLOPs ResNet and a 10 MFLOPs knowledge network at local, we use 40 MFLOPs (30 MFLOPs + 10 MFLOPs) to identify the network capacity we deployed at edge in \proj.

% Commonly, there is a trade off between FL performance and knowledge network size. However, in ablation study~(section \ref{sec:ablation}) we show small knowledge network is an efficient choice. 

%All the baselines are implemented following the non-IID benchmark federated learning setting \cite{li2022niidbench}.

%and FedDF \cite{lin20ensemble} (for model fusion). 

% \input{content/figtex/f_train_effi.tex}

\subsection{Learning Efficiency}
\label{sec:apendix:le}

\begin{figure*}[t]
 \begin{center}

% Resnet50 (res18, res32) (1-2), Mobilenetv3 (res18, res32) (3-4)
\centerline{\includegraphics[width=\linewidth]
{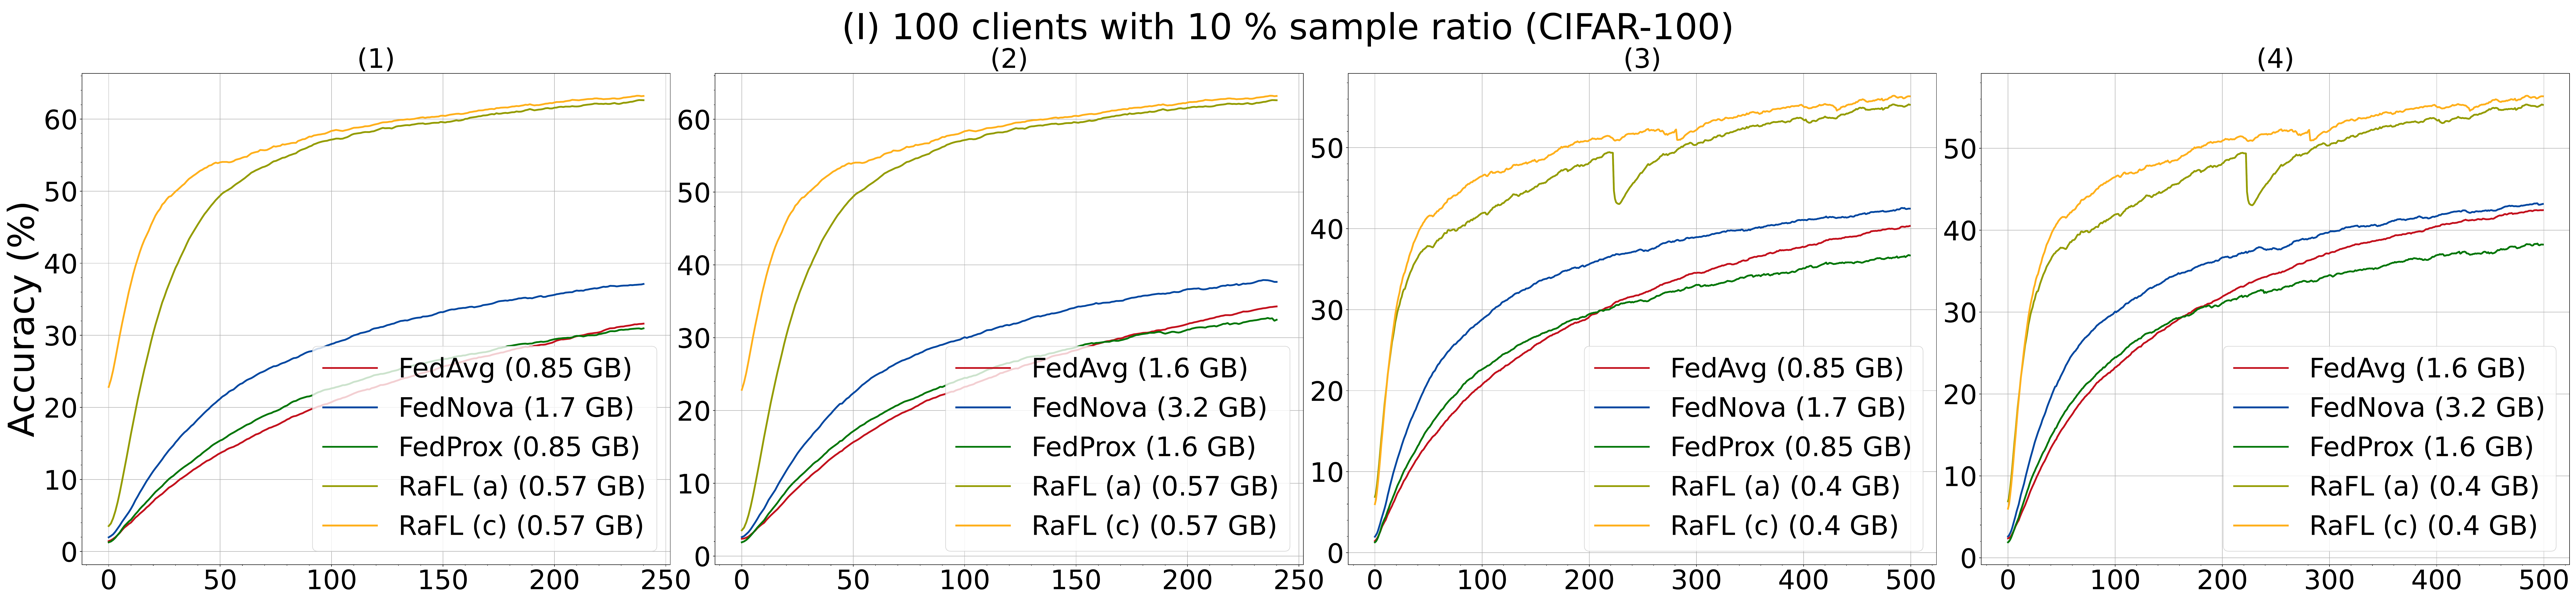}
% {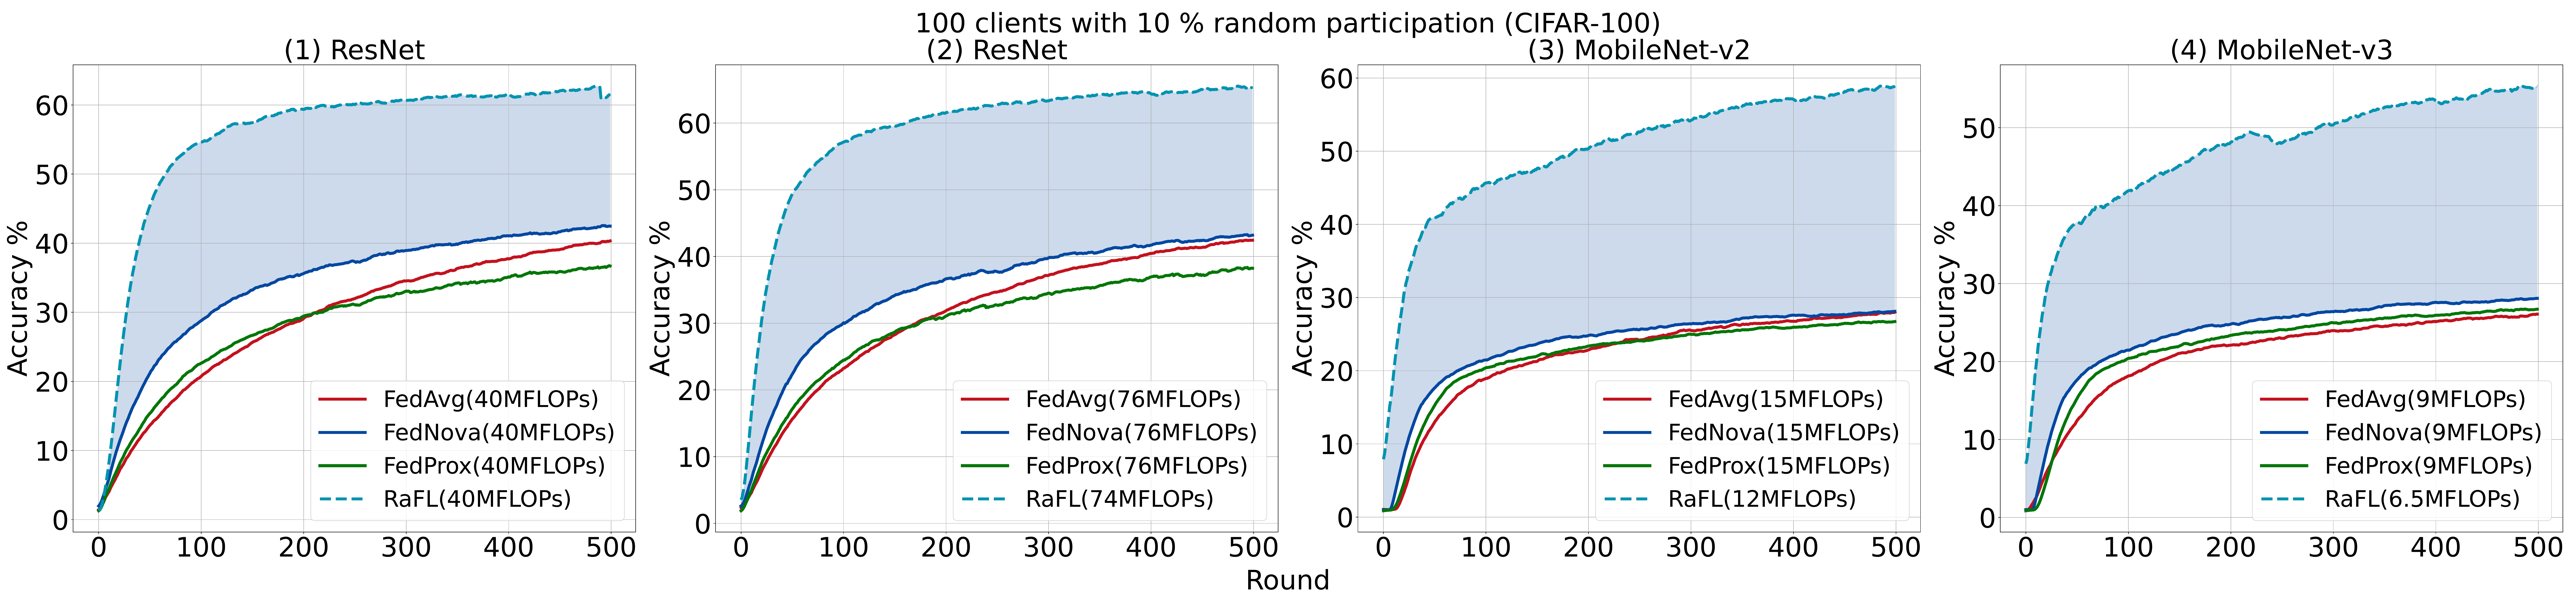}
}
\centerline{\includegraphics[width=1\linewidth]{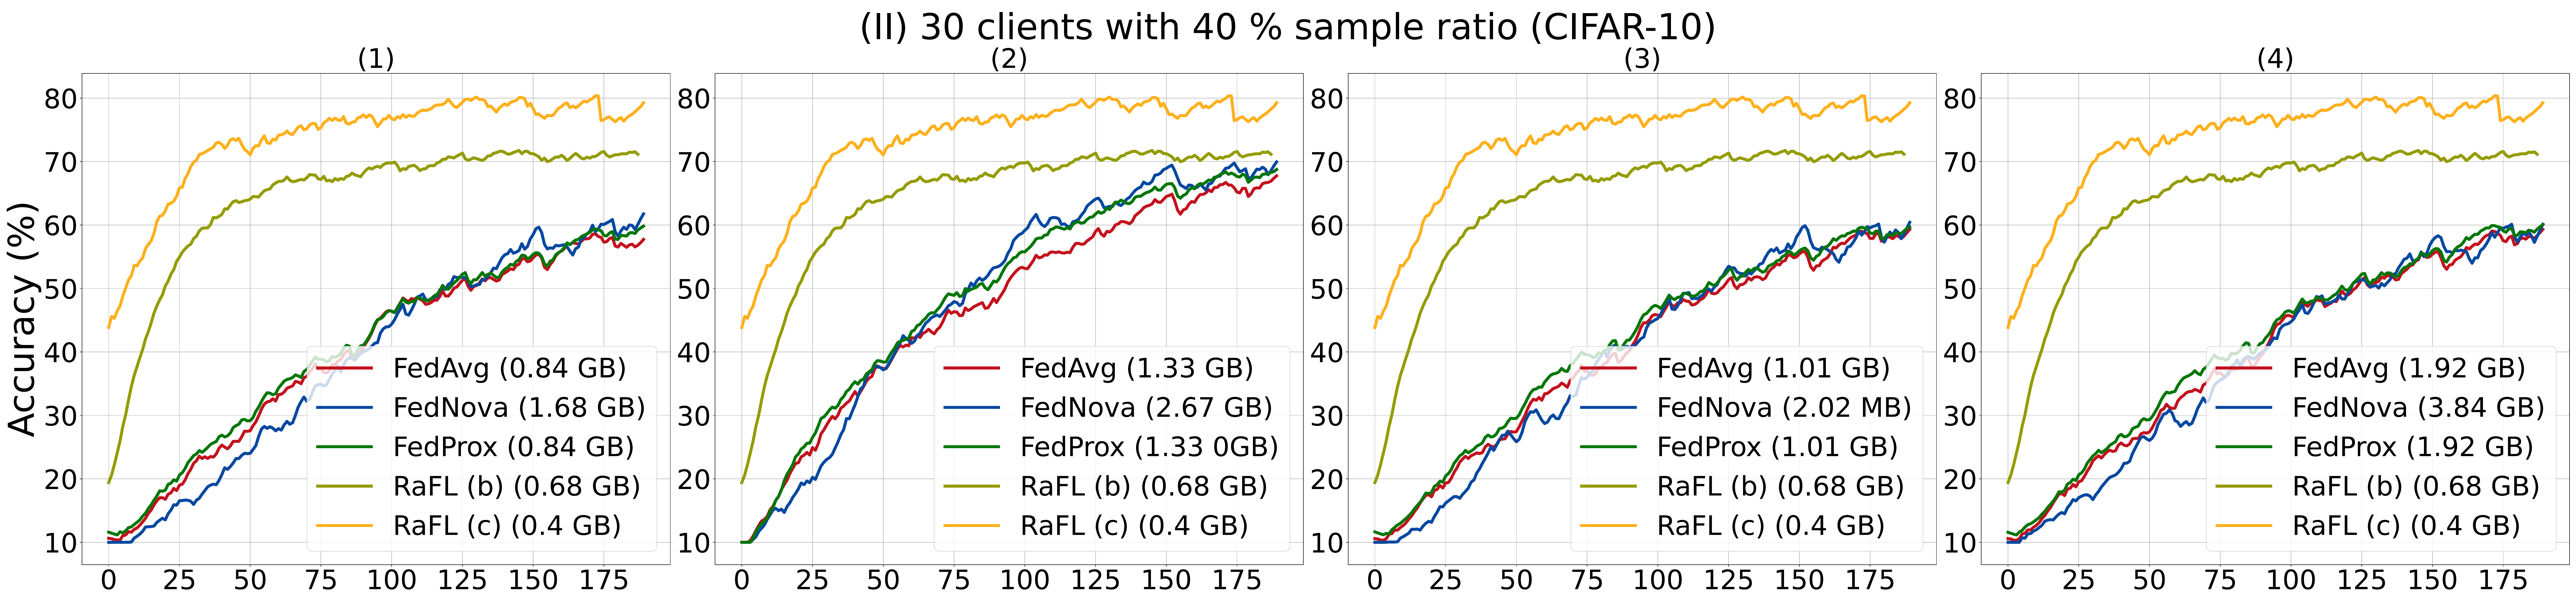}}
% \centerline{\includegraphics[width=1\linewidth]{cvpr2023/Figures/tiny_100_04_ce5_cs15_fused.pdf}}
%avg_100_01_cifar100 % Resnet50(1-2) MobileNetV3(3-4)
% \centerline{\includegraphics[width=\linewidth]{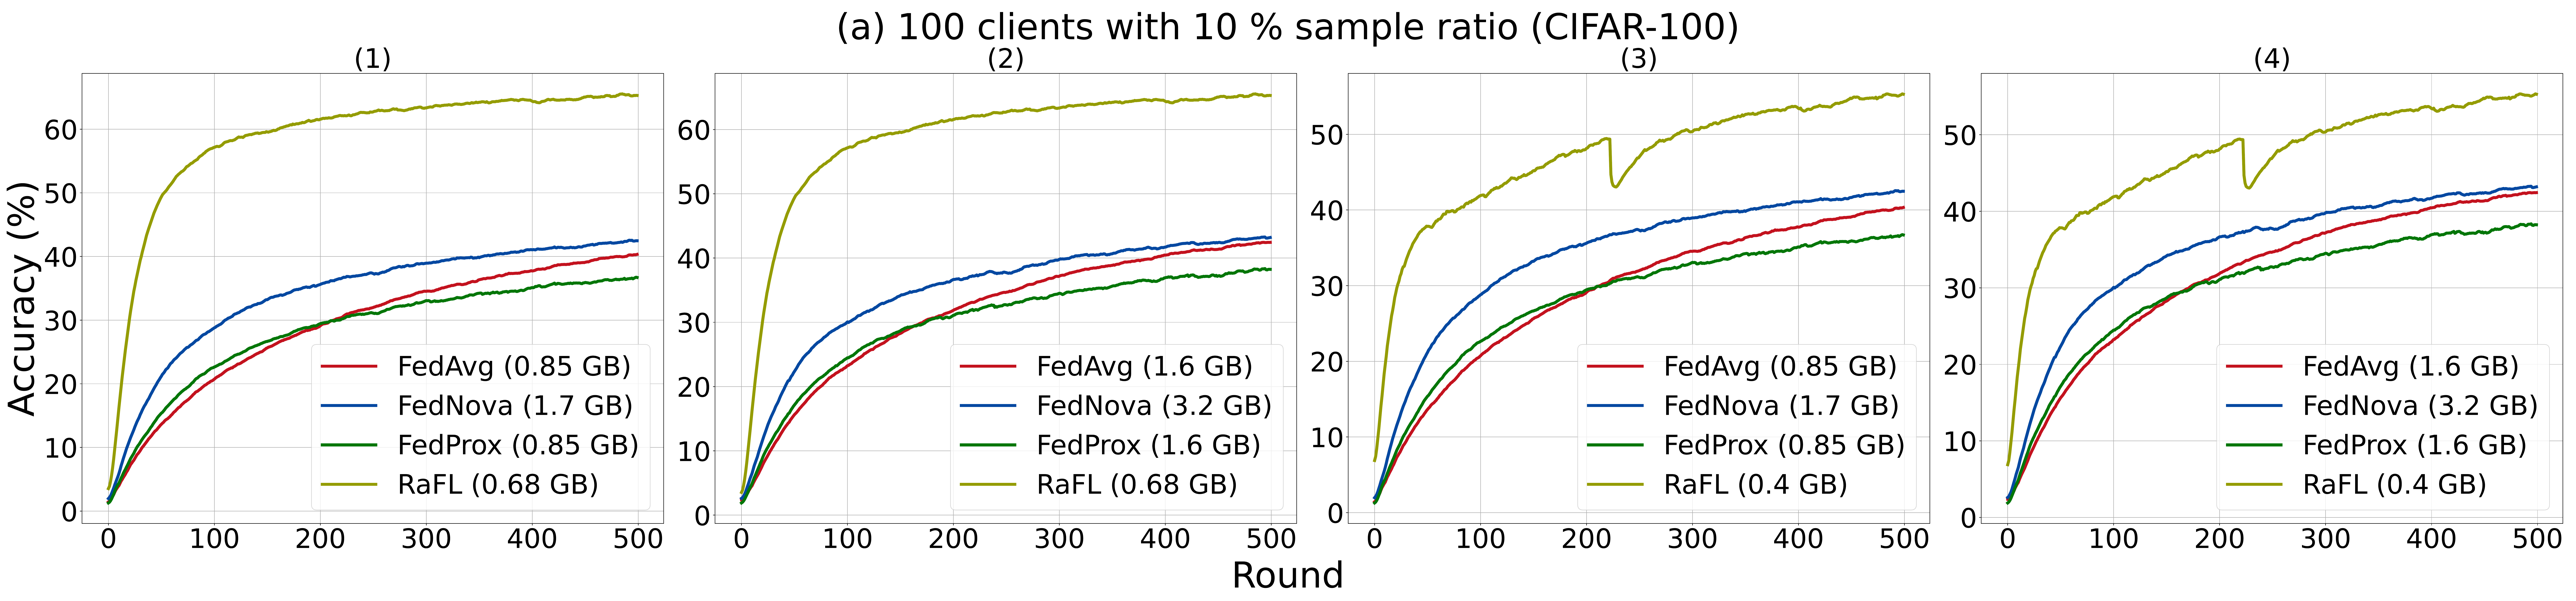}}
% \centerline{\includegraphics[width=1\linewidth]{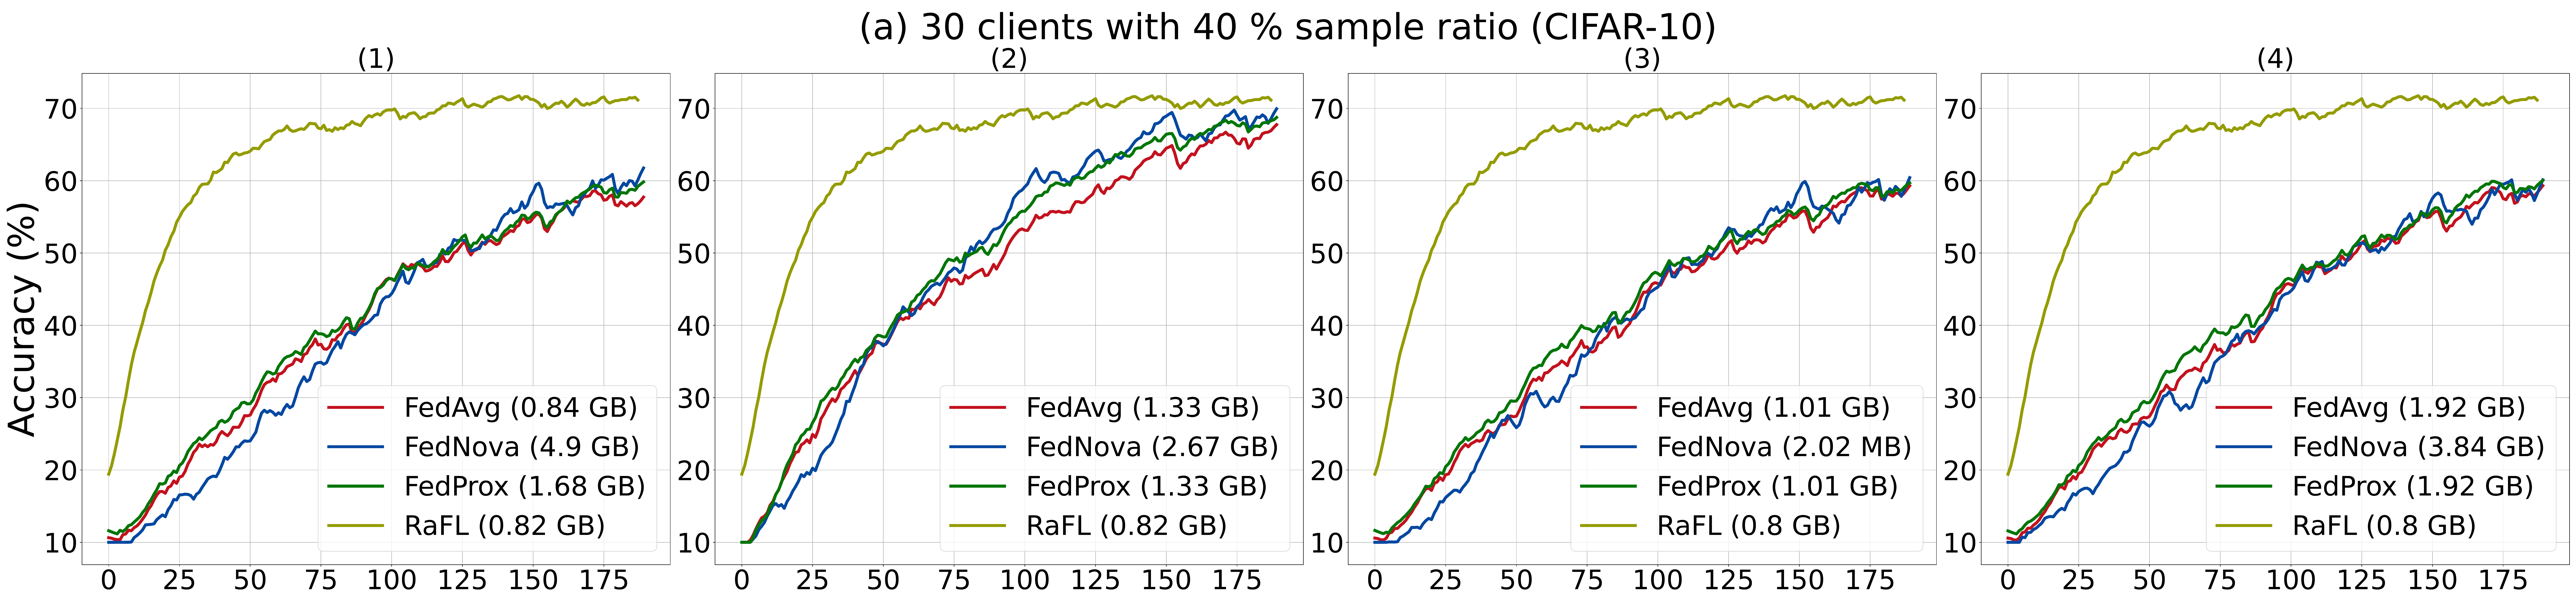}}
% mobilenetv3
% \centerline{\includegraphics[width=1\linewidth]{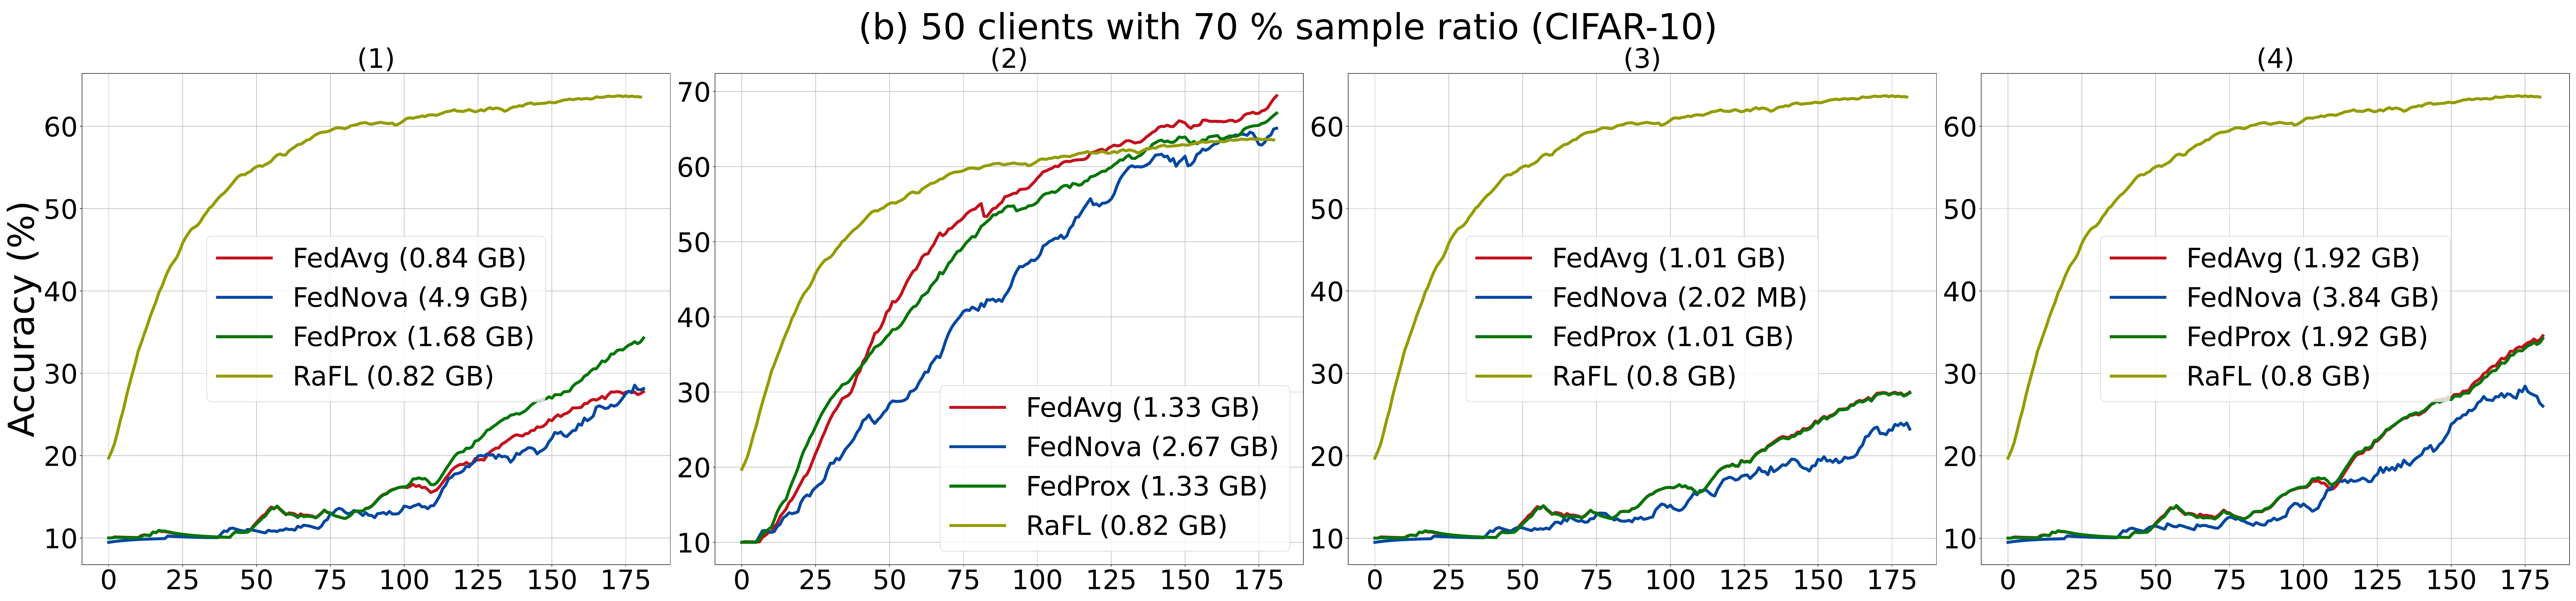}}
% \centerline{\includegraphics[width=1\linewidth]{Figures/tiny_100_04_ce5_cs15_fused.pdf}}
% \centerline{\includegraphics[width=1\linewidth]{Figures/tiny_30_04_ce5_cs15.pdf}}
% mobilenetv3
% \centerline{\includegraphics[width=1\linewidth]{Figures/tiny_50_07_ce5_cs15_mobile.pdf}}
% \centerline{\includegraphics[width=1\linewidth]{Figures/tiny_100_04_ce5_cs15_fused.pdf}}
\caption{Supplementary results: comparison of \proj with SoTAs (numbers in parenthesis represents the communication cost per round).}
\vspace{-1em}
\label{fig:learn_efficiency}
\end{center}
 \end{figure*}
Due to the page limits, in manuscripts, we mainly show the results on CIFAR-100. In this section we provides supplementary results on learning efficiency evaluation, including results on CIFAR-10 and various FL settings.
As shown in Figure~\ref{fig:converge_acc}, we conducted experiments on comprehensive FL settings, from 30 clients to 100 clients and different participating rate. \proj shows stable results and consistently outperform baselines.
Intuitively, Figure~\ref{fig:learn_efficiency} shows training supplementary training logs of \proj.
\proj achieves a higher convergence accuracy while requiring fewer rounds to achieve the target precision compared to baselines. For instance, in the 30 clients FL setting, it ahieves at $70\%$ final accuracy, which is $10\%$ higher than other 3 baselines~(Figure~\ref{fig:learn_efficiency} (II)(1), (II)(3), (II)(4)). There are some exceptions where \proj does not outperform the baselines in case of 100 clients with $40\%$ sample rate (Figure~\ref{fig:learn_efficiency} (II)(3)). \proj with smaller sub-network achieved a converged accuracy of $55\%$, slightly lower than $57\%$ by FedAvg and FedNova. However, it is worth noting that \proj uses far less bandwidth per communication rounds~($1.6$ GB versus $2.8 $GB and $5.6$ GB for FedAvg and FedNova respectively) compared to the baselines. Thus with a small sacrifice in accuracy, we make a larger gain in terms of communication cost.  Compared to the local dataset~(CIFAR10/100), it improves the performance of both the global and local models.

\subsection{Communication Efficiency}
Table~\ref{tab:target_acc} shows the detailed information refers in Figure~\ref{fig:comm_target}. Communicating smaller knowledge network and need fewer rounds to achieve target accuracy help \proj build communication efficient federated leanring.

% % \subsection{Inference acceleration}

% \input{cvpr2023/Tables/t_converged_acc}

\input{cvpr2023/Tables/t_target_acc}

\subsection{Extra burdens of Knowledge Networks}
\label{sec:apdx_extra_kn_cost}
When we initially evaluate \proj, we concerned that adding knowledge network and perform local deep mutual learning might add extra computational burdens at edge.
Hence, we build two FL environments and designed the following experiments:
In the first FL environment, we deployed a 12 MFLOPs MobileNet-V3 and a 8 MFLOPs MobileNet-v3 knowledge network at every single local client.
In the second FL environment, we deployed a 20 MFLOPs MobileNet-V3, at every single local client, and directly local update the model with SGD algorithm without the knowledge distillation.
To make a relatively fair comparison, and avoid any lottery results, we train the above two FL environments 500 rounds separately in the same nodes and the same type of GPU (NVIDIA v100s). Since our experimental platform is an HPC server, other jobs running on the HPC ontology might affect the actual training time, and a few deviations may present, but it is acceptable. 
We surprisingly found that the second FL setting takes 49 hours and 19 minutes, while the first FL setting takes 48 hours and 25 minutes to finish training, even faster than only optimizing a single model.
We further consult an expertise researcher in related areas, the reason is: when we perform deep mutual learning on the local model (12 MFOLOPs network) and knowledge network (8 MFLOPs network), our python deep learning framework will create a corresponding computational graph for each network and load in memory, and use them for gradient calculation. We can view the two computational graphs as disconnected computational graphs. Hence, training a disconnected computational graph (with a 12 MFLOPs sub-graph and 8 MFLOPs sub-graph) takes a similar computational cost as we train a single 20 MFLOPs computational graph.
\input{cvpr2023/Tables/t_kd.tex}

\subsection{Comparison with KD-based FL}
\label{sec:apdx_kdbaselines}
In our experiment, as Table~\ref{tab:kd_baselines} shows, we found that using knowledge distillation to aggregate local models may not improve the FL's learning efficiency. The performance of knowledge distillation highly depends on the similarity of public data and local data. Pure knowledge distillation does not apply to all general FL environments.
In this section, we compare \proj with knowledge distillation baseline FedDF~\cite{lin2020feddf} under different public data.
FedDF aggregates local models by ensemble local models and distillates the ensemble knowledge to the global model. \proj is more robust, in each round of communication, \proj first initializes the global knowledge network by weighted averaging local knowledge networks via Equation~\ref{eq:aggre}, and then optionally performs ensemble knowledge distillation. In case the public data drifts significantly from the overall local data distribution in FL, \proj can suffer less negative effects.
% However, ensemble knowledge distillation doesn’t always
% improve performance. It’s dependent on the similarity of
% the public and private client data distributions

\subsection{Analysis \proj and other FL NAS method}
\label{sec:apdx_nas}
In this section, we analyze the pros and cons of mainstream NAS methods in FL with RaFL, such as FedNAS~\cite{he2020fednas} and DecNAS~\cite{xu2020decnas}.
Firstly, we have different objections. Both FedNAS~\cite{he2020fednas} and DecNAS~\cite{xu2020decnas} target to optimize the NAS super-network via federated learning on user private data. FedNAS deploy NAS super-networks to every local client and perform NAS before local updating. Then each client updates a sub-network derived from the local NAS super-network and aggregate local sub-networks to the corresponding part of the super-network in the cloud. Similarly, DecNAS aims to optimize NAS super-network in a decentralized manner and utilize data and computational resources at the edge. 

Both of the methods may not get efficient neural architecture. For instance, in NAS, the search process usually starts after the super-network is well-trained, and it requires us to maintain a look-up table to track high-performance architectures under certain resource constraints.
However, FedNAS perform a neural architecture search at the very beginning of the training, and it may not get high-performance architectures.
Second, existing methods may not efficiently address resource heterogeneity at the edge. existing methods only consider the inference when in applications, and they directly deployed supernet at the edge. For example, FedNAS directly perform neural architecture at the edge. Neural architecture search is computationally costly, which may not fit resource constraints edge devices. 
Lastly, optimizing super-networks in FL environments are easily leading to divergence. It may work when the number of clients is limited. Nevertheless, when the FL becomes large-scale, for instance, 100 clients on CIFAR-100 in our experiments, where each client only allocated 500 data points, it's almost impossible to converge the over-parameterized super-networks. In our experiments, we show that our baselines suffer remarkably over fittings.  

In RaFL, we ingeniously avoid the above limitations, we dynamically deploy specialized high-performance networks to edge clients based on their local resource overhead.  Clients with the resource-aware model deployment can efficiently utilize their local resources and enable better downstream tasks.
% \subsection{Ablation Study}
% \subsection{Effect of knowledge network size}
% \subsection{Effect of Network capacity}
% \subsection{Effect of cloud algorithm}
